# Supplementary material for: Online Multi-modal Person Search in Videos
Source: arXiv:2008.03546 source file (2020-08-08)
Supplement: Supplementary file 1 [file supp.tex]

% !TEX root = ../main.tex

\clearpage
